# Supplementary material for: A novel experimental system for the KDK measurement of the $^{40}$K decay scheme relevant for rare event searches
Source: arXiv:2012.15232 source file (2021-07-27)
Supplement: Supplementary file 1 [file Appendix_Conversion_Electrons.tex]

\newpage
\section{\label{App:Conversion_Electrons}Conversion Electrons (Not For Publication)}

When a nucleus decays through electron capture it is possible (and usually the case) that the decay proceeds to an excited state of the daughter nucleus. The nuclear de-excitation to ground state can then occur through two competing process: internal conversion or gamma emission. Internal conversion is when the the energy from the excited state is given to a shell electron causing it to escape from the nucleus. The energy of the escaping electron will be the excited state transition energy minus the binding energy of the shell the electron escaped from. If the nuclear transition energy is above 1022~keV internal electron-positron pair formation (IPF) is possible. 

The internal conversion coefficient ($\alpha_i$) is defined as the ratio of electrons (N$_i$) ejected from the i$^{th}$ shell, over the number of gammas emitted (N$_\gamma$) when a nuclear de-excitation occurs~\cite{band_diracfock_2002}. This is shown in Eq.~\ref{Eqn:ICC},

\begin{equation}\label{Eqn:ICC}
    \alpha_i = \frac{N_i}{N_\gamma}.
\end{equation}

The total internal conversion coefficient (ICC, $\alpha_T$) is the sum of all individual ICC for each shell in the nucleus.

\begin{equation}\label{Eqn:Total_ICC}
    \alpha_T  = \sum_i \alpha_i
\end{equation}

So the probability of a conversion electron being produced instead of a gamma emission is $\alpha_T/ (1+\alpha_T)$. For our purposes the ICC are calculated using~\cite{band_diracfock_2002,kibedi_evaluation_2008}, specifically the no-holes approximation.

\subsection{\label{App:Mn_ICC} Mn-54 ICC}

\begin{table}[ht]
\centering
\begin{tabular}{cl}\hline
Shell & $\alpha_i$ \\\hline
Tot. & 0.000275 (4)  \\
K & 0.000249(4) \\
L & 0.0000234(4)\\
M & 0.00000318 (5)\\
N & 0.0000001522(22) \\\hline

\end{tabular}
\caption[]{\label{tab:mn54_ICC} Calculated ICC from~\cite{kibedi_evaluation_2008} for \Mn. The no-holes approximation was used. K-shell dominates.}
\end{table}

The effect of Internal conversion was considered in the likelihood when the gamma tagging efficiency was evaluated for the 835~keV transition from \Mn, see Section~\ref{subsec:Efficiency} for details on this. Information about the likelihood derivation can be found in Lilianna's document \textit{Effect of SDD Tagging-Efficiency of Conversion Electrons in KDK Analysis}. The overall effect was found to be larger than (by a factor of 5) statistical uncertainty found for the efficiency. For this reason the effect of conversion electrons were included in the likelihood analysis, see~\ref{App:Mn54_Efficiency_Model}. For example when we calculated the efficiency without considering conversion electrons we got 0.9776(1) for 2$~\mu$s. When conversion electrons were considered the value was 0.9781(1), see Table~\ref{tab:Modular_Efficiency}. 

\subsection{\label{App:Zn_ICC} Zn-65 ICC}
 
\begin{table}[ht]
\centering
\begin{tabular}{cl}\hline
Shell & $\alpha_i$ \\\hline
Tot. & 0.000203(3)  \\
K &  0.000181(3)\\
L & 0.0000180(3)\\
M & 0.00000258(4)\\
N &  0.0000001045(15)\\
IPF & 0.000000920(13) \\\hline

\end{tabular}
\caption[]{\label{tab:Zn65_ICC} Calculated ICC from~\cite{kibedi_evaluation_2008} for \Zn. The no-holes approximation was used. K-shell dominates.  IPF (Internal Pair Formation) starts to appear.}
\end{table}

For \Zn, the effect of conversion electrons is small relative to statistical limitations. Here, the parameter of interest is $\rho = I_{EC}/I_{EC*}$, which is close to unity at all coincidence windows. The statistical error on all obtained values of $\rho$ is around $\sigma = 0.015\%$, and including conversion electrons in the analysis varies the results at the $\sim 0.3\sigma$ level. Preliminarily, at the 1-$\mu$s coincidence window $\rho = 0.9782(15)$ in the no-conversion-electron approximation, and $\rho = 0.9786(15)$ otherwise. For small $\alpha_T$, $\rho \propto \alpha_T$, and thus including conversion electrons in the analysis slightly increases $\rho$.

\subsection{\label{App:K_ICC} K-40 ICC}

\begin{table}[ht]
\centering
\begin{tabular}{cl}\hline
Shell & $\alpha_i$ \\\hline
Tot. & 0.0001078(15)  \\
K &  0.0000308(5)\\
L & 0.00000258(4) \\
M & 0.000000280(4)\\
N & 0.0000000101(15)\\
IPF & 0.0000741(11) \\\hline

\end{tabular}
\caption[]{\label{tab:K40_ICC} Calculated ICC from~\cite{kibedi_evaluation_2008} for \K. The no-holes approximation was used. IPF (Internal Pair Formation) dominates.}
\end{table}

Although, we have not yet analyzed the effect of conversion electrons on \K\ we can perform a back of the envelope calculation to determine the number of expected conversion electrons in our data set. N.B. This is a preliminary analysis and conclusion more work will be done on the actual effect of conversion electrons on \K, but save that for a later paper. From our $\sim$ 33 day run we measured roughly 47000 \ECStar events. This was determined from a fit on the coincident SDD spectrum, see~\ref{Fig:K40_Coinc_Spec_Fit.png}. The fit determined the number of K$_\alpha$ and K$_\beta$ events that were seen, of which both internal conversion and gamma emission will contribute. The coincidence spectrum had no energy cuts on the MTAS spectrum.

If we assume that 47000 is the total number of detected \ECStar\ events, using Table~\ref{tab:K40_ICC} we know that of the 47000, $\sim$5 (47000$\times$0.0001078 = 5.066) of these events will have been conversion electrons. The dominant mode of internal conversion for \K\ will actually be pair production which releases two 511~keV gammas which can be detected in MTAS with a similar efficiency to the 1460~keV~\cite{karny_modular_2016}. This implies that the conversion electrons will likely be classified into the coincident spectrum. 46995 gamma events are detected with a statistical uncertainty of $\pm$ 216. The number of conversion electron are 43 times lower than the statistical uncertainty on the gamma electron capture events. 

If, all the conversion electrons fall in the anti-coincidence signal region, they will be competing with two primary backgrounds: 1) The $\beta-$ background which has 32618 $\pm$ 180  events in the 2.5-3.5~keV range. 2) \ECStar\ whose gammas were not tagged which results in false positives. Based on the efficiency from Table~\ref{tab:Final_Corrected_Efficiency} that is 969 $\pm$ 31 events. In case 1 the conversion electrons are 36 times lower than the statistical uncertainty of the $\beta-$ background and in case 2, they are 6 times lower. The above calculations imply that even if we missed tagging the conversion electrons they would not be the dominant source of background in the experiment. For the above reasons I (Matt) think we can ignore conversion electrons in the \K\ analysis. The chance of the conversion electron itself making it into MTAS is small 2.7$\%$ calculated from Geant simulations.

\begin{figure}[ht]
    \includegraphics[width=1.0\textwidth]{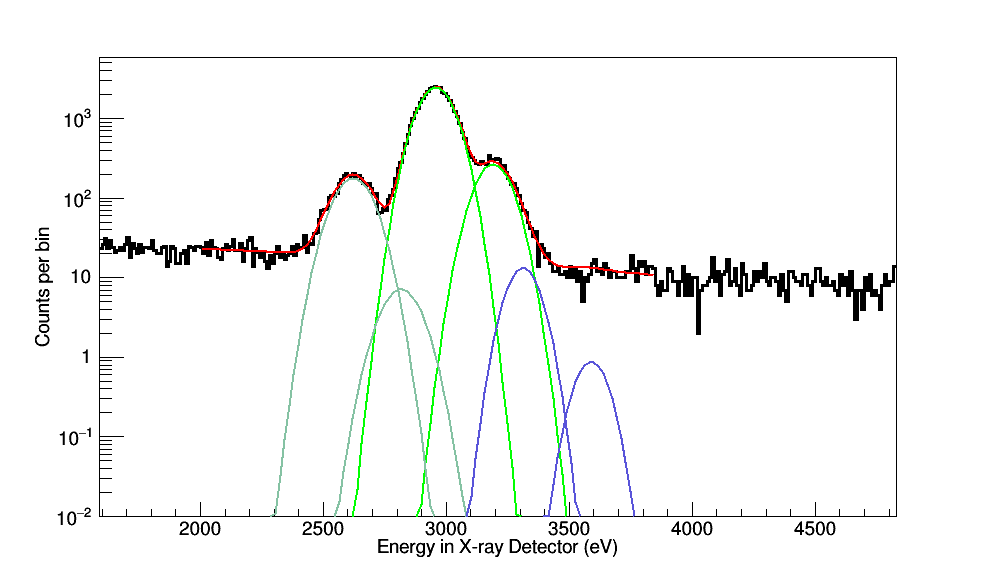}
    \centering
	\caption{\label{Fig:K40_Coinc_Spec_Fit.png}Fit of the \K, 4~$\mu$s CW, coincident spectrum. Data is shown in black. K$_\alpha$ and K$_\beta$ from the Ar of the \K\ decay are the light green lines. A total of $\sim$47000 counts were measured under the green lines. Cl fluorescence are the grey lines and K fluorescence are the blue lines. }
\end{figure}
