# Supplementary material for: A novel experimental system for the KDK measurement of the $^{40}$K decay scheme relevant for rare event searches
Source: arXiv:2012.15232 source file (2021-07-27)
Supplement: Supplementary file 2 [file Appendix_For_Geant.tex]

\section{Appendix for section~\ref{subsec:Geant_Simulations} (Not For Publications) \label{App:Geant_Sims}}

\begin{figure}[ht]
    \includegraphics[width=0.5\textwidth]{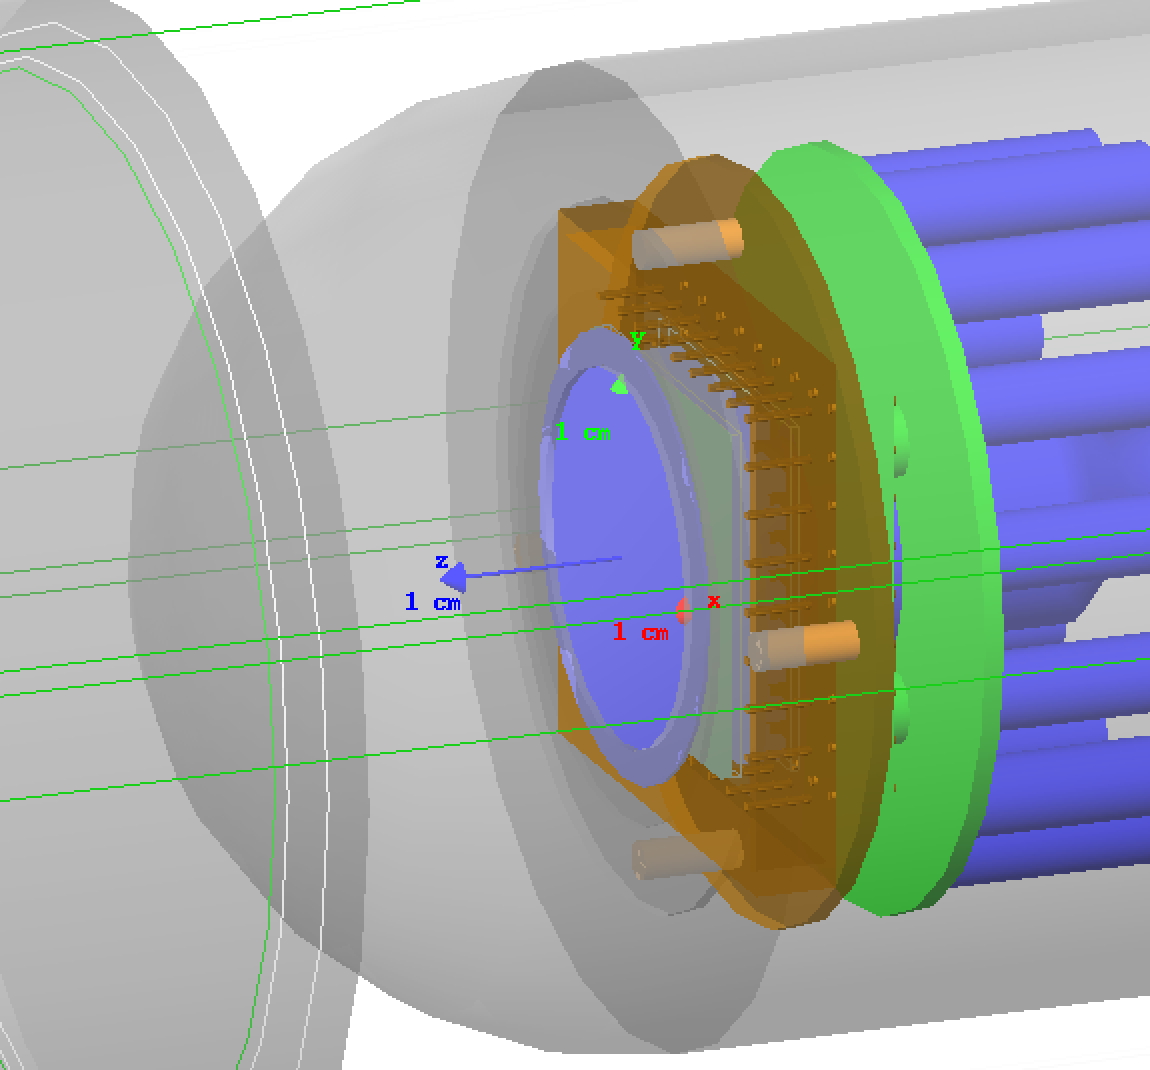}
    \centering
	\caption{\label{Fig:Geant_Sim_1.png}Geant 4 modelling of the SDD inside the MTAS module.}
\end{figure}

\begin{figure}[ht]
    \includegraphics[width=1.0\textwidth]{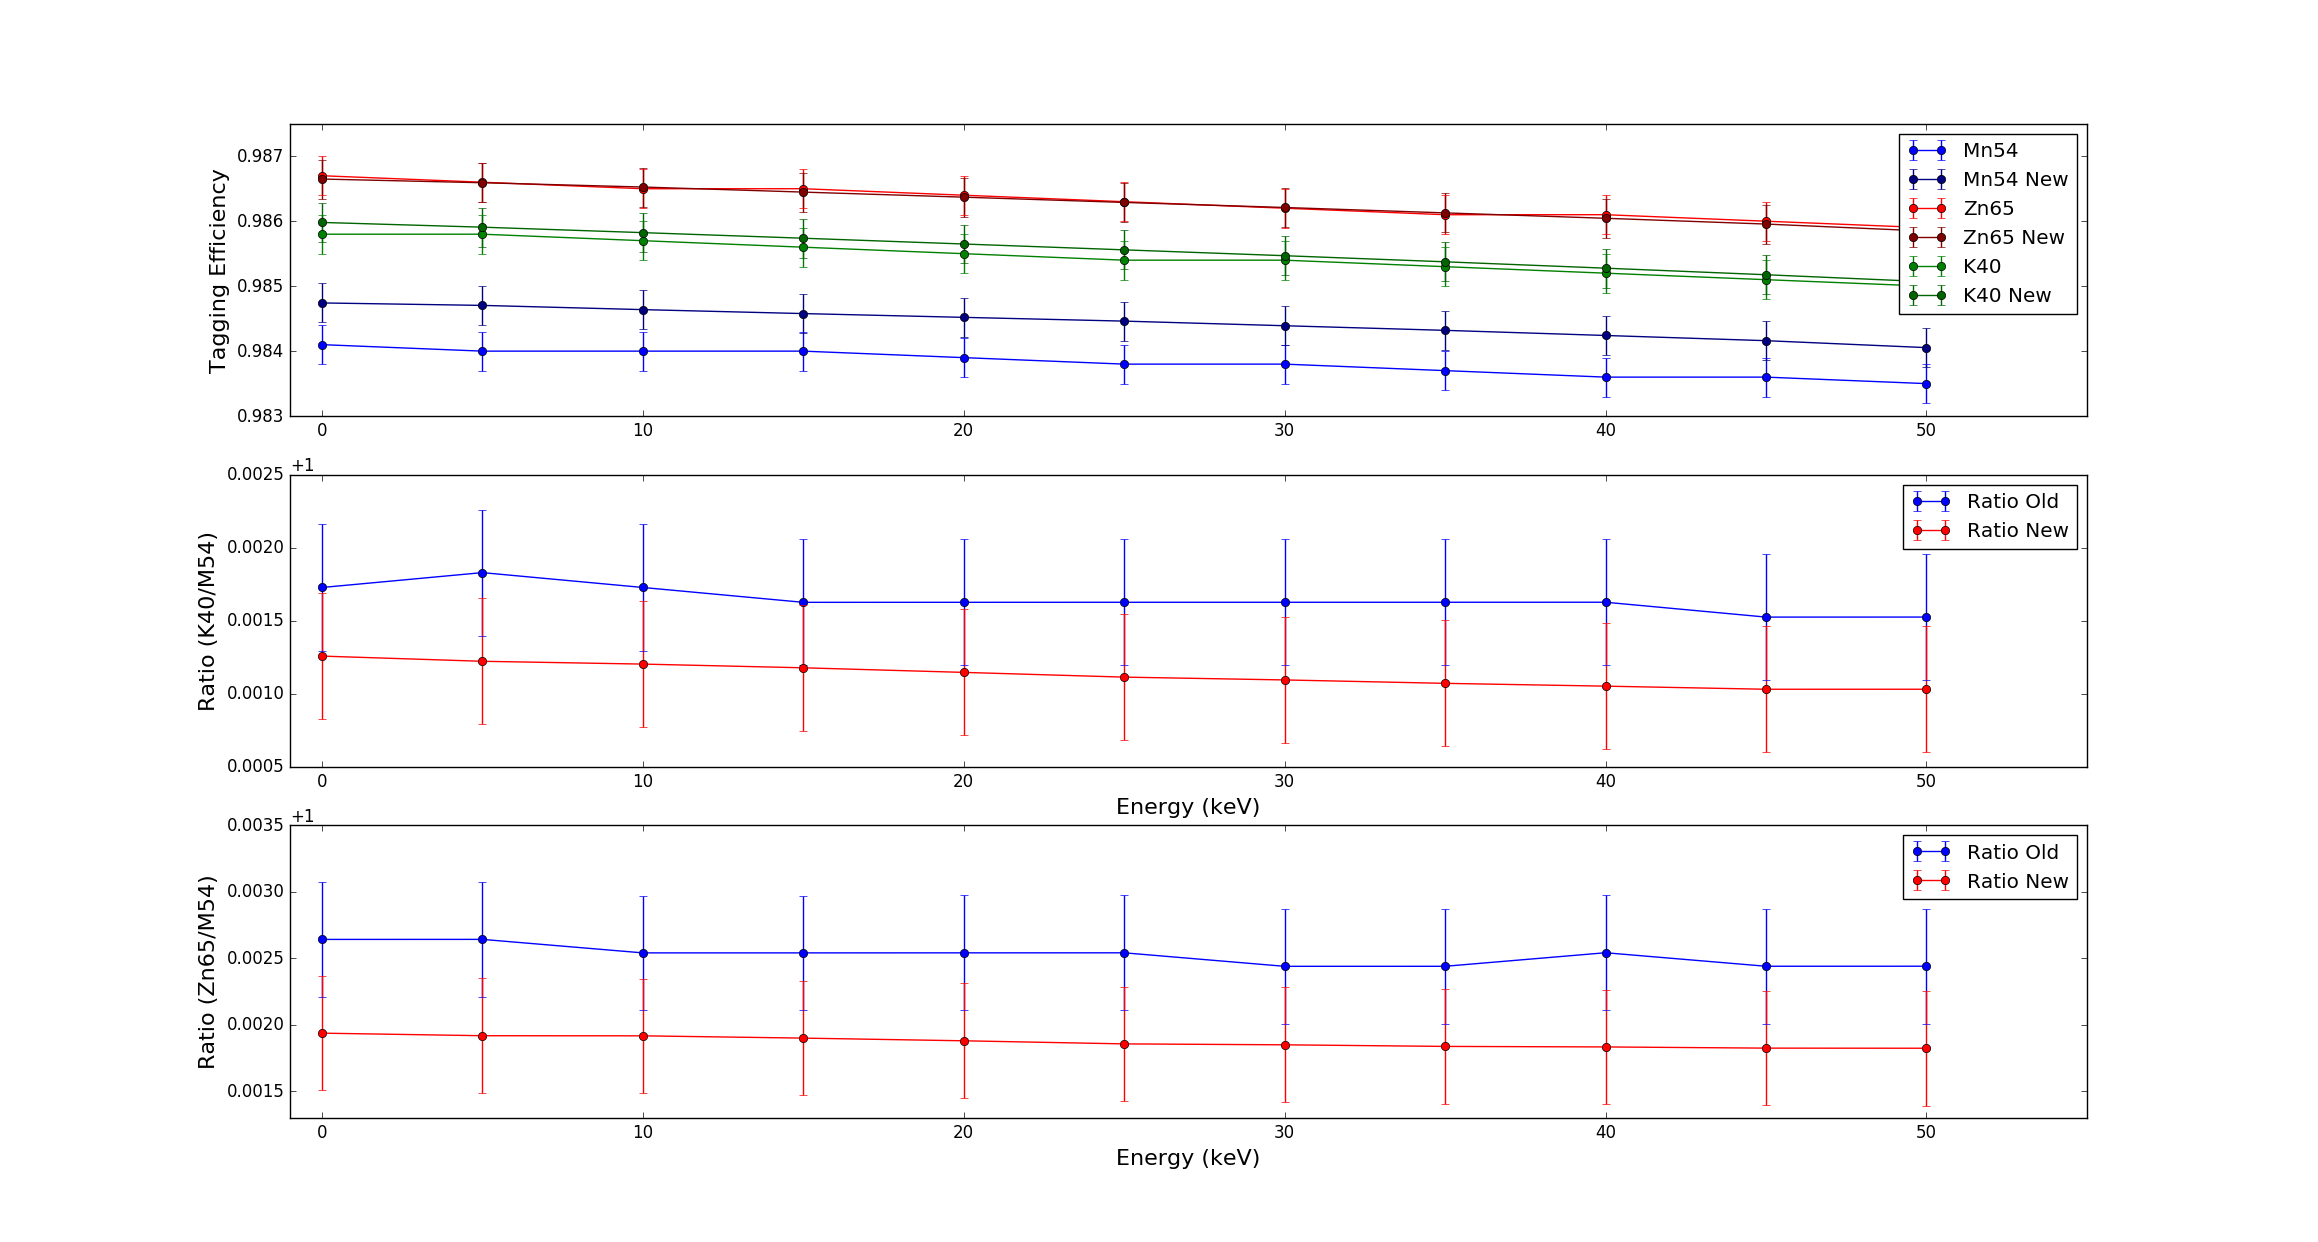}
    \centering
	\caption{\label{Fig:Energy_Threshold_Comparison.png}Shows the simulated tagging efficiency as a function of energy threshold for three different source (\K, \Zn~and \Mn). The legends detail New vs. Old which refers to the testing of different physics lists. Energy threshold is the value above which the depositions into MTAS are counted. The ratio between source is shown in the inserts. The ratio is within one standard deviation when the physics lists are changed and is independent of the low energy threshold selected.}
\end{figure}

\begin{figure}[ht]
    \includegraphics[width=1.0\textwidth]{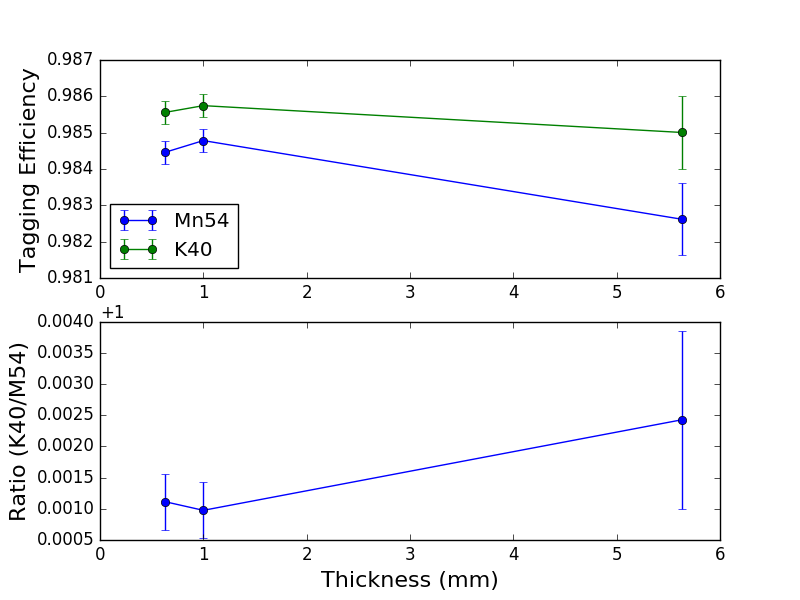}
    \centering
	\caption{\label{Fig:Efficiency_vs_Thickness_Comparison.png}Shows the tagging efficiency as a function of thickness of the aluminum cap that surrounds the source. The nominal thickness is 0.63mm and the ratio is independent with a dactor of 2 increase.  }
\end{figure}

\begin{figure}[ht]
    \includegraphics[width=1.0\textwidth]{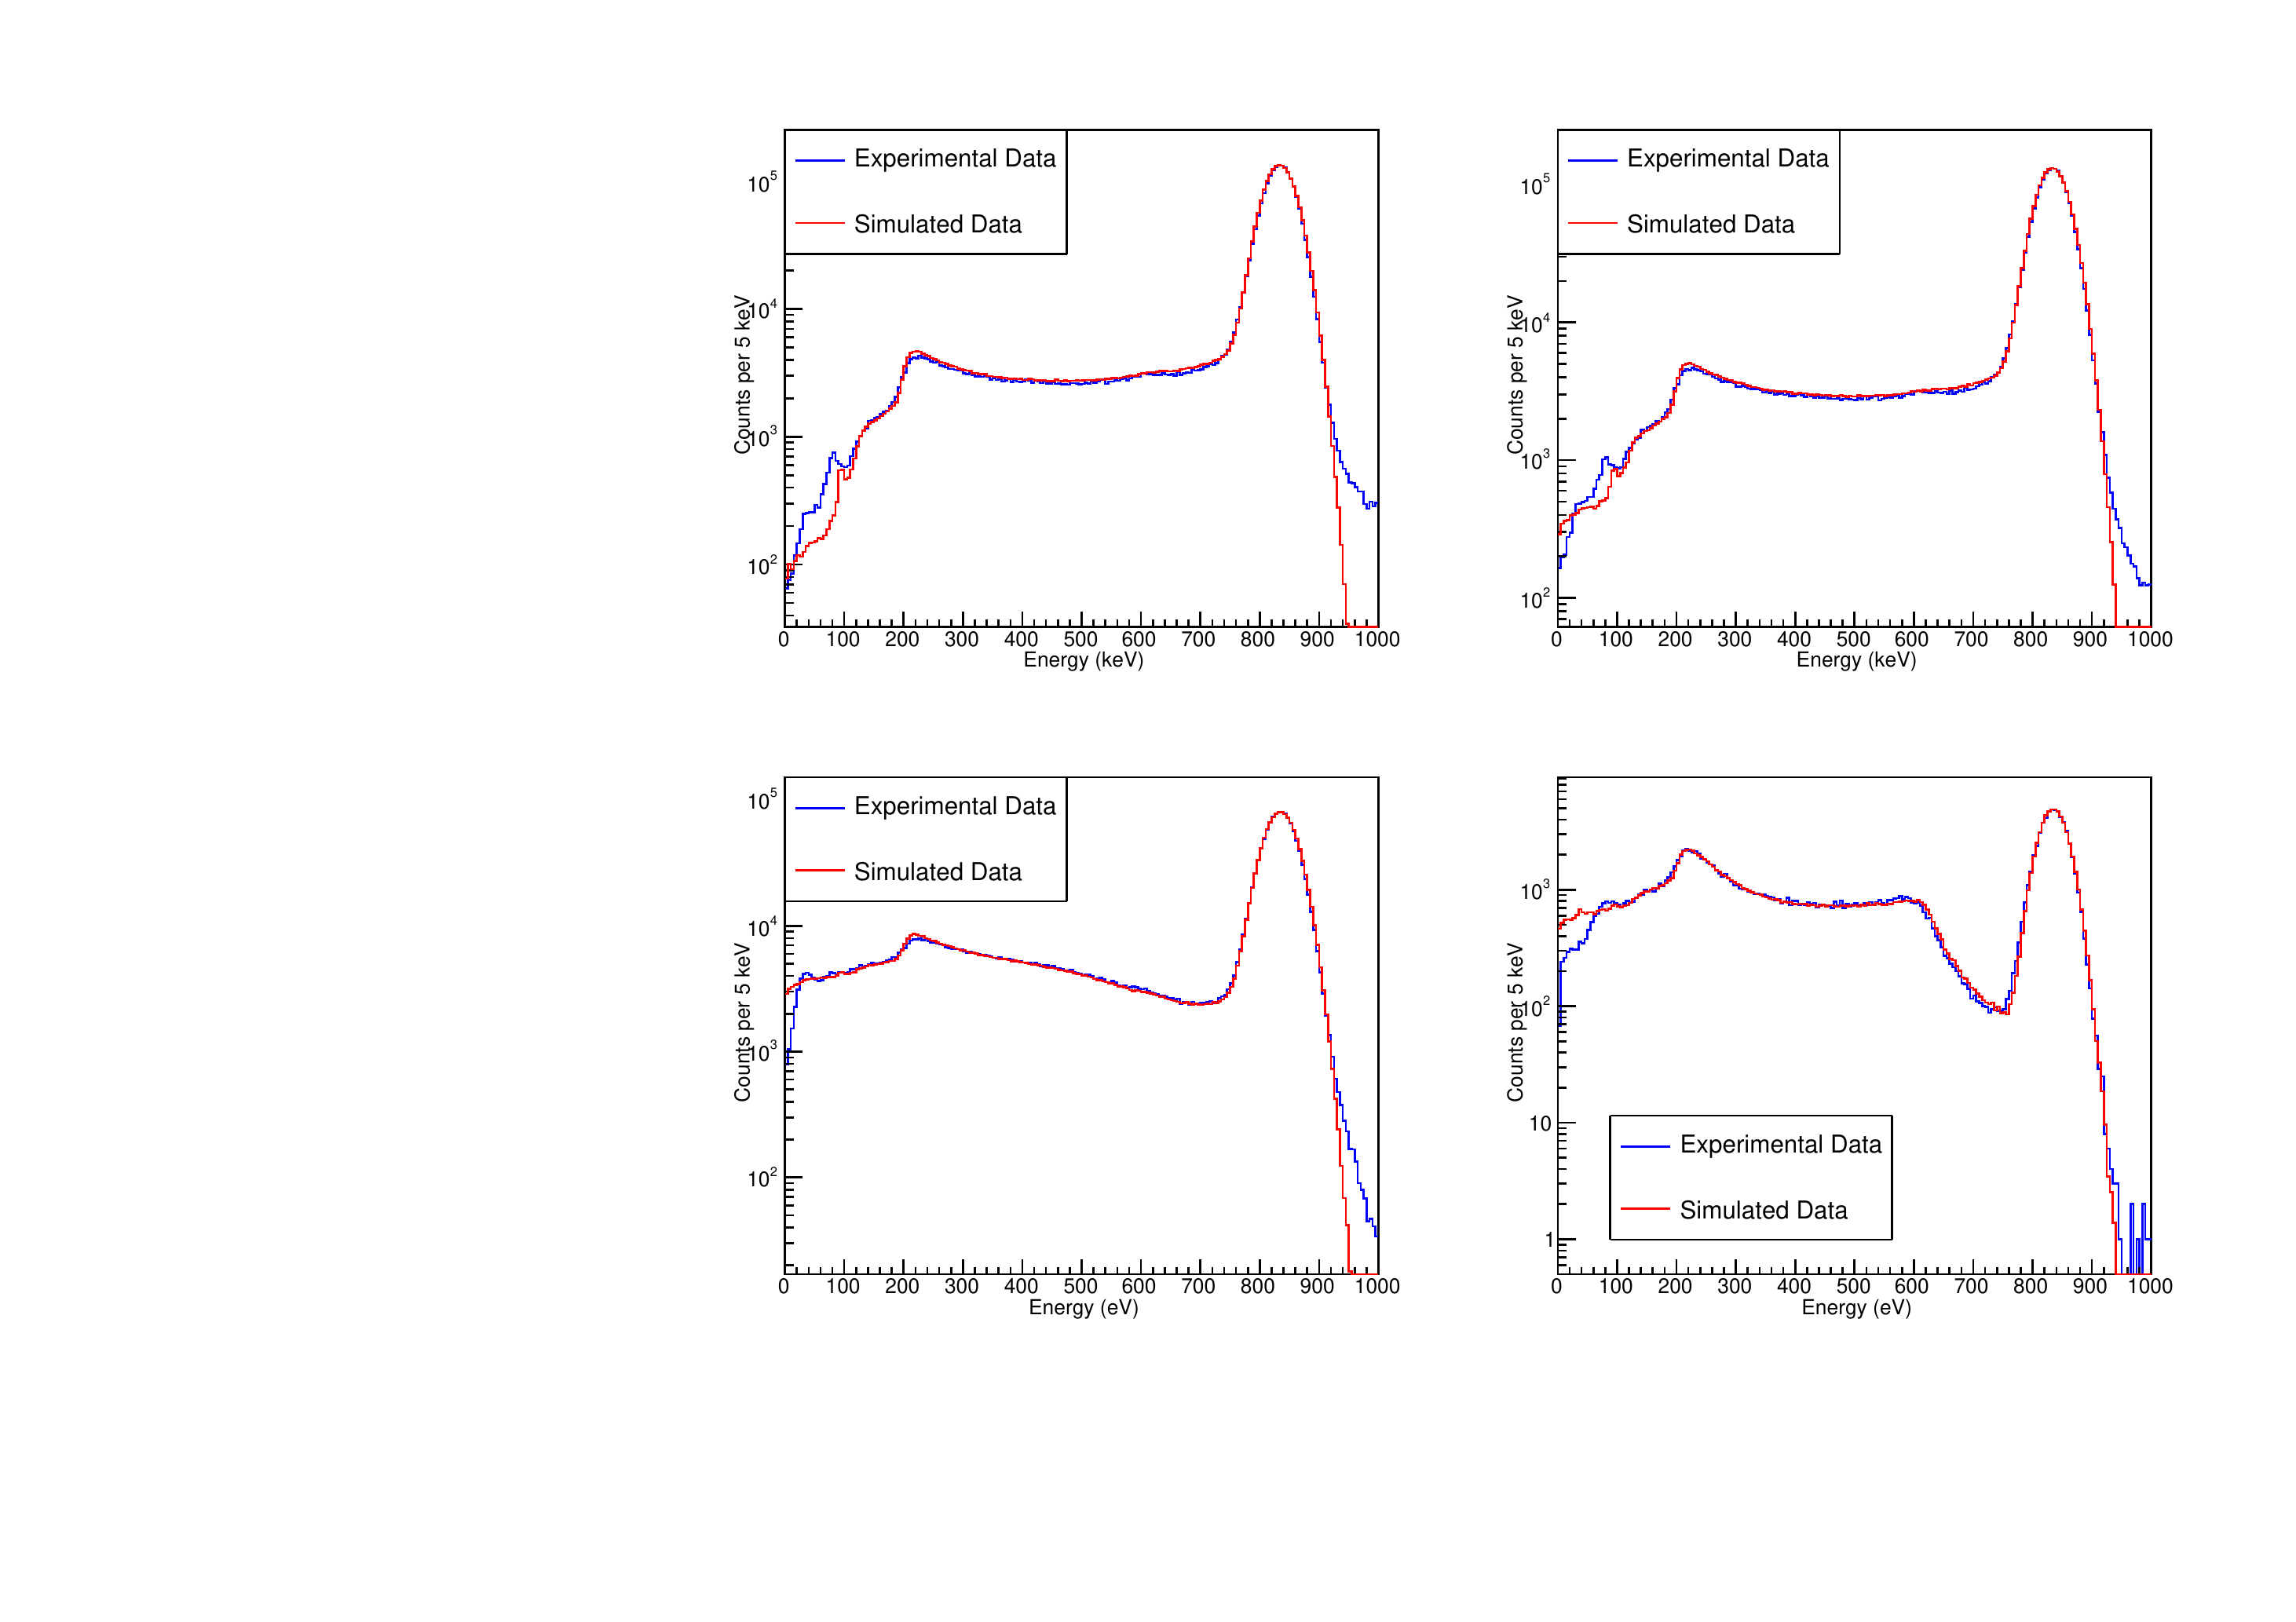}
    \centering
	\caption{\label{Fig:Geant_Sim_2.png} Comparison of \Mn~gamma spectrum in MTAS when triggered by the SDD (blue) versus Geant 4 simulated spectrum (red). The comparison is done when considering four different combinations of MTAS. Top Left: Centre, Inner, Outer, Middle and Plug (ie Total) of MTAS. Top Right: Centre, Inner and Plug. Bottom Left: Centre and Plug of MTAS. Bottom Right: Plug of MTAS.  See text for discussion of low and high energy behavior.}
\end{figure}

\begin{figure}[ht]
    \centering
    \includegraphics[width=\textwidth]{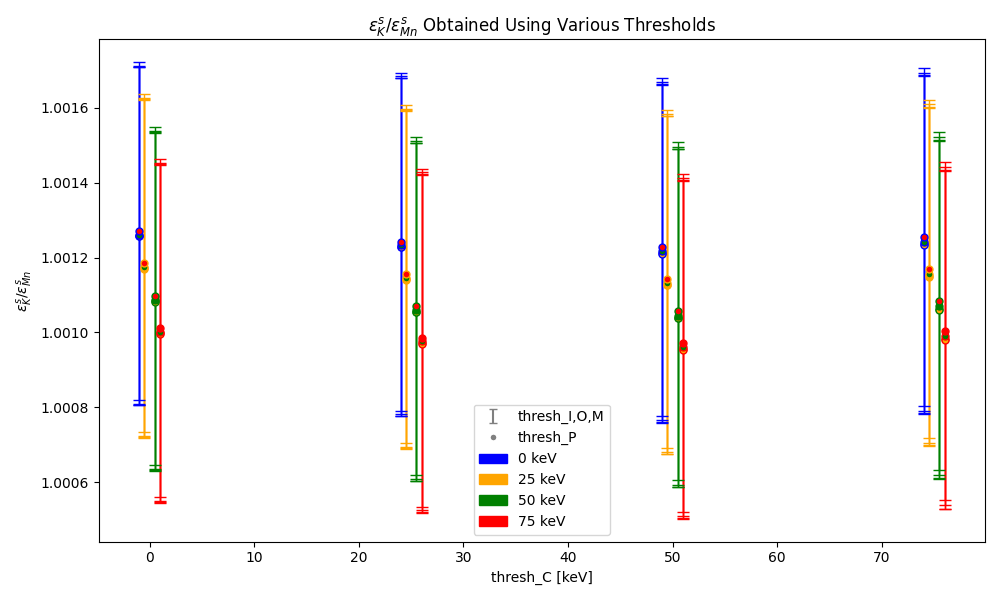}
    \includegraphics[width=\textwidth]{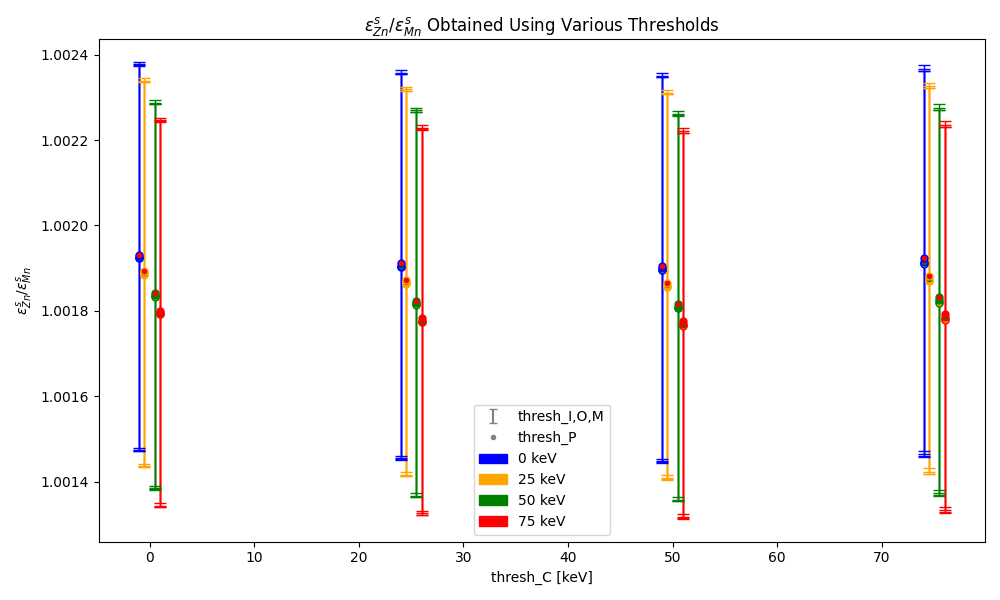}
    \caption{Simulated efficiency ratios $\varepsilon^s_K/\varepsilon^s_{Mn}$ and $\varepsilon^s_{Zn}/\varepsilon^s_{Mn}$ obtained using various combinations of energy thresholds. Values are plotted against the threshold of the center ring, ``thresh\_C". For each data point, the errobar colour details the threshold applied to the inner, outer, and middle rings (``thresh\_I,O,M"), while the marker colour specifies the plug threshold (``thresh\_P"). Values were obtained at various combinations of the thresholds \keV{0}, \keV{25}, \keV{50}, \keV{75}. Data are offset from their true thresh\_C values for clarity. Errors are solely statistical.}
    \label{Fig:app_geant_sims:efficiency_ratio_K_thresholds}
\end{figure}
