# Supplementary material for: A novel experimental system for the KDK measurement of the $^{40}$K decay scheme relevant for rare event searches
Source: arXiv:2012.15232 source file (2021-07-27)
Supplement: Supplementary file 3 [file Appendix_For_live_time.tex]

\section{Appendix for section~\ref{subsec:Dead Time Considerations}(Not For Publications)\label{App:Dead_Time}}
For this experiment we use Pixie-16 Digital Gamma Finder (DGF) pulse shape processing spectrometer cards from XIA, as well as acquisition and analysis software co-developed by personnel at the University of Tennessee and Oak Ridge National Laboratory over the last 15 years.

\subsection{Pixie-16 DAQ from XIA \label{ssec:DAQ}}

The general description of the acquisition is rather completely described in the manual from XIA \cite{xia_llc_pixie-16_2009}. In this section, the particulars of the implementation of the acquisition for the MTAS Detector is described.  

The cards themselves are based on the CompactPCI/PXI standard and are organized to first receive the signal, condition the signal via resistive elements and a Nyquist filter, to sample and digitize the signal based on a 100 MHz clock, to handle logical processes in a Field Programmable Gate Array (FPGA), and then handle Digital Signal Processing (DSP) in a trapezoidal filtering scheme in order to reliably extract energy and time information. The signals are digitized by 12-bit ADCs, pulse heights are calculated to 16 bit precision and can be binned into spectra with 32K bins. The output data rate along the backplane and to the acquisition computer is reliable with a single shared timestamp below data rates of 109 Mbyte/s. Data rates during the 40K run were typically near 150 kbyte/s. 

The version numbers of the XIA provided firmware used are 32495 (FPGA), 33157(Communication), and 32777 (Configuration). 

The acquistion is run in a self-triggered list mode. Events are written to a file which contains the trigger time (time stamp) of all pulses on all channels. Traces of the signal are also recorded for the SDD. Acquisition parameters are tabled below. The header includes the energy, time, and channel specification along with boolean values which are true if there was a signal pileup condition met or if the signal recorded was out of the range of the digitizer.

The events written to the file are processed to determine coincidences. The software which scans the data files offline can be found publicly at 

\href{url}{https://github.com/ntbrewer/pixie\_ldf\_slim}. The coincidence window, $dt$, is a global, rolling coincidence window.

The software hosted there is for the KSI segment of the KDK collaboration but is identical for the details of MTAS processing. 

There are four physical pathways to consider for our acquisition.
\begin{enumerate}
    \item Channel
    \item Channel Group (4 channels)
    \item Pixie Module (16 channels, 4 groups)
    \item Crate
\end{enumerate}

It is important to note that there are no sources of dead-time for the channel group or for the Pixie Module. Our data rates were 2-3 orders of magnitude smaller than the level were this would be a real issue. Furthermore, this would be a global loss rate and could not affect the ratio of EC/EC*. Channel level effects, then, are the only dead times to consider.

There are three sources of acquisition dead-time and three sources of processing dead-time to consider for this experiment.

Acquisition:
\begin{enumerate}
    \item In the digital signal processing (DSP)
    \item From the length of the trace
    \item From the shaping time
\end{enumerate}

Processing:
\begin{enumerate}
    \item Signal Pile-up rejection
    \item Incomplete Center Module events
    \item Event Pile-up rejection
\end{enumerate}

By a similar argument as above, acquisition dead-times only related to the SDD (i.e. related to traces and shaping) do not impact the EC/EC* ratio because both EC and EC* require an SDD trigger.  Therefore the DSP dead-time is the only issue to consider in depth. The DSP dead time can be calculated from the count rate. 

All of the processing dead-times can be directly counted because they are in the data. A signal pile-up is when there are two triggers coming from the timing filter within the envelope of the energy filter. Event pile-up is when the same MTAS module has two or more events in the span of the coincidence window. There is also dead time associated with the multiplicity of events in the center module of MTAS. Since there are 12 PMTs connected to a single crystal, it is expected that all 12 should trigger simultaneously. If there is a center multiplicity less than 12, the event energy is scaled by 12 divided by the multiplicity. The energy of the central modules are adjusted further in our gain match procedure. Therefore the dead time resulting from losing channels in the central module is not effecting the efficiency.

All of these remaining dead-times can be modeled as the 'paralyzable' type.  This means that each occurrence of the situation leading to dead-time will prolong the length of the dead-time. This model means that the Output Count Rate (OCR) is related to the Input Count Rate ($ICR$) and the Dead Time ($dt$) by the formula $OCR = ICR * exp^{-ICR * dt }$. This function is invertable with the use of the Lambert-W function as $ICR = W(-dt * OCR) / -dt $. The dead-time percentage can then be calculated as $ (1 - OCR/ICR)*100\%$. Average measured rates ($OCR$) in the SDD and various rings of MTAS are shown in Table \ref{tab:Rate_Table}. The most important point of these rates is that the rates for Mn and for K are very similar. The dead-time effect works like a rate dependent efficiency and it can be sufficient to show that the minimal change in rate results in a minimal change in efficiency. After an explanation of what the DSP is doing, values are shown for the various dead-times.

\begin{table}[ht]
\centering
\begin{tabular}{c|c|c|c|c|c|c}
Isotope & \multicolumn{6}{c}{Average Counting Rates (Hz)}\\
 & Plug & Central & Inner & Middle & Outer & SDD \\\hline
88Y & 225 & 1545 & 381 & 219 & 211 & 239   \\
65Zn & 27.6 & 309 & 174 & 198 & 204 & 46.5 \\
54Mn & 18.4 & 217 & 166 & 200 & 206 & 29.9 \\
40K &  12.7 & 160 & 159 & 196 & 202 & 11.9 \\
\end{tabular}
\caption[Rate Table]{\label{tab:Rate_Table_c} Table of rates (Hz) in various detector segments during measurements of different sources.}
\end{table}

Values used in our experiments are shown in Table \ref{tab:Filter_Values}. In this table RISETIME refers to the length of the filter window and FLATTOP refers to the length of the distance between them. 

\begin{table}[ht]
\centering
\begin{tabular}{c|c|c|c}
Parameter Name & \multicolumn{3}{c}{Value ($\mu$s)}\\
 & MTAS (CIMO) & Plug & SDD \\\hline
ENERGY\_RISETIME & 2 & 0.56 & 0.48 \\
ENERGY\_FLATTOP & 0.48 & 0.24 & 2 \\
FILTER\_RISETIME & 0.6 & 0.6 & 0.3 \\
FILTER\_FLATTOP & 0.3 & 0.01 & 0.01 \\
Tau & 0.94 & 0.15 & 8 \\
TRACE\_LENGTH & & & 12\\
TRACE\_DELAY & & & 5
\end{tabular}
\caption[Filter Value Table]{\label{tab:Filter_Values} Table of values for the trapezoidal filters used for the on-board analysis of various detectors.}
\end{table}

\begin{table}[ht]
	\centering
	\begin{tabular}{c|c|c|c|c|c}
\multicolumn{5}{c}{Rates (Hz) for various experimental runs}\\
Module  & BKG & 40K & 54Mn & 65Zn & 88Y \\\hline
C  & 172.06(3) & 164.07(3) & 213.04(3) & 290.30(4) & 1232.25(8)\\
I  & 172.46(3) & 164.57(3) & 169.53(3) & 177.21(3) & 358.32(4) \\
M  & 201.24(3) & 197.40(3) & 199.32(3) & 197.70(3) & 217.31(3) \\
O  & 212.86(3) & 209.88(3) & 211.97(3) & 209.55(3) & 216.98(3) 
	\end{tabular}
	\caption[Rate Table]{\label{tab:Rate_Table_2} Table of rates (Hz) in various detector segments during measurements of different sources.}
\end{table}

Now making these tables with an exclusive condition, I find live time correction factors as follows:

\begin{table}[ht]
	\centering
	\begin{tabular}{c|c|c|c|c|c}
		\multicolumn{5}{c}{Live-time due to Signal Pile-up rejection}\\
		Module  & BKG & 40K & 54Mn & 65Zn & 88Y \\\hline
	 C  1 us & 99.71(3) & 99.70(3) & 99.76(2) & 99.82(2) & 99.93(1) \\
		2 us & 99.66(3) & 99.67(3) & 99.74(2) & 99.80(2) & 99.92(1) \\
		4 us & 99.63(3) & 99.65(3) & 99.73(2) & 99.79(2) & 99.92(1) \\
	 I  1 us & 99.90(3) & 99.90(3) & 99.90(3) & 99.90(2) & 99.94(2) \\
		2 us & 99.87(3) & 99.87(3) & 99.87(3) & 99.88(3) & 99.93(2) \\
		4 us & 99.85(3) & 99.85(3) & 99.85(3) & 99.86(3) & 99.91(2) \\
	 M  1 us & 99.66(2) & 99.70(3) & 99.68(3) & 99.65(2) & 99.66(2) \\
		2 us & 99.64(2) & 99.69(3) & 99.67(3) & 99.64(2) & 99.64(2) \\
		4 us & 99.63(2) & 99.69(3) & 99.66(3) & 99.63(2) & 99.62(2) \\
	 O  1 us & 99.56(2) & 99.55(3) & 99.55(3) & 99.54(3) & 99.54(2) \\
		2 us & 99.56(2) & 99.55(3) & 99.55(3) & 99.54(3) & 99.53(2) \\
		4 us & 99.56(2) & 99.55(3) & 99.55(3) & 99.54(3) & 99.52(2)
	\end{tabular}
	\caption[Signal pile-up rejection]{\label{tab:Signal_PUR} Table of live-time percentages for various modules during runs measuring various isotopes due to signal pile-up rejection. }
\end{table}

\begin{table}[ht]
	\centering
	\begin{tabular}{c|c|c|c|c|c}
		\multicolumn{5}{c}{Live-time due to Event Pile-up rejection}\\
		Module  & BKG & K & Mn & Zn & Y \\
C  1 us & 100.00(2) & 100.00(3) & 100.00(2) & 100.00(2) & 100.00(1) \\
   2 us & 100.00(2) & 100.00(3) & 100.00(2) & 100.00(2) & 100.00(1) \\
   4 us & 99.97(2) & 99.97(3) & 99.97(2) & 99.96(2) & 99.84(1) \\
I  1 us & 100.00(2) & 100.00(2) & 100.00(2) & 100.00(2) & 100.00(2) \\
   2 us & 100.00(2) & 100.00(3) & 100.00(2) & 100.00(2) & 100.00(2) \\
   4 us & 99.94(2) & 99.97(3) & 99.97(3) & 99.97(2) & 99.94(2) \\
M  1 us & 100.00(2) & 100.00(2) & 100.00(2) & 100.00(2) & 100.00(2) \\
   2 us & 100.00(2) & 100.00(2) & 100.00(2) & 100.00(2) & 100.00(2) \\
   4 us & 99.94(2) & 99.97(2) & 99.97(2) & 99.97(2) & 99.94(2) \\
O  1 us & 100.00(2) & 100.00(2) & 100.00(2) & 100.00(2) & 100.00(2) \\
   2 us & 100.00(2) & 100.00(2) & 100.00(2) & 100.00(2) & 100.00(2) \\
   4 us & 99.96(2) & 99.98(2) & 99.98(2) & 99.98(2) & 99.95(2)
	\end{tabular}
	\caption[Event pile-up rejection]{\label{tab:Event_PUR} Table of live-time percentages for various modules during runs measuring various isotopes due to event pile-up rejection.}
\end{table}

\begin{table}[ht]
	\centering
	\begin{tabular}{c|c|c|c|c|c}
		\multicolumn{5}{c}{Calculated live-time due to DSP hold-up}\\
		Module  & BKG & 40K & 54Mn & 65Zn & 88Y \\\hline
		C  & 99.91462(1) & 99.91859(1) & 99.89428(2) & 99.85591(2) & 99.38692(4) \\

		I  & 99.91442(1) & 99.91834(1) & 99.91588(1) & 99.91206(1) & 99.82212(2) \\
		
		M  & 99.90014(2) & 99.90204(2) & 99.90109(2) & 99.90189(2) & 99.89216(2) \\
		
		O  & 99.89437(2) & 99.89585(2) & 99.89481(2) & 99.89601(2) & 99.89232(2)
	\end{tabular}
	\caption[DSP live time]{\label{tab:DSP} Table of calculated live-time percentages for various modules during runs measuring various isotopes due to DSP processing hold-up.}
\end{table}

\begin{table}[ht]
\centering
\begin{tabular}{r|l|l|l|}
		\multicolumn{4}{c}{Calculated Total Live-Time}\\
Module $dt$ &  K  &	 Mn 	& Zn\\
C  1 us & 99.70(4) & 99.76(3) & 99.82(3) \\
   2 us & 99.67(4) & 99.74(3) & 99.80(3) \\
   4 us & 99.63(4) & 99.70(3) & 99.75(3) \\
I  1 us & 99.81(4) & 99.81(4) & 99.82(3) \\
   2 us & 99.79(4) & 99.79(4) & 99.79(3) \\
   4 us & 99.74(4) & 99.74(4) & 99.74(4) \\
M  1 us & 99.61(3) & 99.58(3) & 99.55(3) \\
   2 us & 99.59(3) & 99.57(3) & 99.54(3) \\
   4 us & 99.56(4) & 99.53(3) & 99.50(3) \\
O  1 us & 99.45(4) & 99.45(3) & 99.44(3) \\
   2 us & 99.45(4) & 99.44(4) & 99.43(3) \\
   4 us & 99.42(4) & 99.42(4) & 99.41(3)
\end{tabular}
\caption[Correction Factors]{\label{tab:CorrFactors} CIMO, MTAS ring live time percentages}
\end{table}

%Zn STILL PRELIMINARY UNTIL AFTER MATT DISCUSSES IC.
\begin{table}[ht]
\centering
\begin{tabular}{r|c|c|c|c|}
		\multicolumn{5}{c}{Factors Used For Efficiency Determination}\\
 & $dt$ &  Mn  &	 K 	& Zn \\
Uncorrected Efficiency 	&	1us 	 & 0.9776(1)  & 0.9854(3)  & 0.9781(15) \\
			&	2us 	 & 0.9779(1)  & 0.9792(4)  & 0.9766(15) \\
			&	4us 	 & 0.9782(1)  & 0.9794(4)  & 0.9774(15) \\
 Efficiency Factor 	&	1us 	 & 0.9977(7)  & 1.0004(8)  & 0.9995(17) \\
			&	2us 	 & 0.9974(7)  & 1.0005(8)  & 0.9995(17) \\
			&	4us 	 & 0.9970(7)  & 1.0005(9)  & 0.9995(17) \\
Corrected Efficiency 	&	1us 	 & 0.9799(7)  & 0.9850(8)  & 0.9786(16) \\
			&	2us 	 & 0.9804(7)  & 0.9787(8)  & 0.9771(16) \\
			&	4us 	 & 0.9811(7)  & 0.9789(8)  & 0.9779(16) \\
Ratio Mn/Isotope 	&	1us 	 & 1.0000(7)  & 0.9972(8)  & 0.9981(17) \\
			&	2us 	 & 1.0000(7)  & 0.9969(8)  & 0.9979(17) \\
			&	4us 	 & 1.0000(7)  & 0.9965(9)  & 0.9975(17) 
\end{tabular}
\caption[Efficiency Factors DT]{\label{tab:EffFactorsDT} MTAS effeciency correction factors changing with respect to coincidence window}
\end{table}

\begin{table}[ht]
\centering
\begin{tabular}{r|c|c|c|}
		\multicolumn{4}{c}{Factors Used For Efficiency Determination}\\
 & Module &  Mn  &	 K 	\\
Uncorrected Efficiency 	&	CP  	 & 0.8235(3)  & 0.7454(3) \\
			&	CIP  	 & 0.9713(1)  & 0.9627(3) \\
			&	CIMOP  	 & 0.9779(1)  & 0.9788(3) \\
 Efficiency Factor 	&	CP  	 & 0.9976(5)  & 1.0006(6) \\
			&	CIP  	 & 0.9977(5)  & (6) \\
			&	CIMOP  	 & 0.9977(7)  & 1.0004(8) \\
Corrected Efficiency 	&	CP  	 & 0.8255(4)  & 0.7450(4) \\
			&	CIP  	 & 0.9736(5)  & 0.9623(6) \\
			&	CIMOP  	 & 0.9802(7)  & 0.9784(8) \\
Ratio Mn/Isotope 	&	CP  	 & 1.0000(5)  & 0.9970(6) \\
			&	CIP  	 & 1.0000(5)  & 0.9973(6) \\
			&	CIMOP  	 & 1.0000(7)  & 0.9972(8) 
\end{tabular}
\caption[Efficiency Factors Module]{\label{tab:EffFactorsMod} MTAS effeciency correction factors changing with respect to Module}
\end{table}

\begin{table}[ht]
\centering
\begin{tabular}{rcccc}\hline
		\multicolumn{5}{c}{Factors Used For Efficiency Determination}\\
 & $dt$ &  Mn  &	 K 	& Zn \\\hline
Live-Time  	&	1us 	 & 0.9977(7)  & 1.0004(8)  & 0.9995(17) \\
Correction Factor			&	2us 	 & 0.9974(7)  & 1.0005(8)  & 0.9995(17) \\
			&	4us 	 & 0.9970(7)  & 1.0005(9)  & 0.9995(17) \\
Ratio Mn/(K,Zn) 	&	1us 	 &   & 0.9972(8)  & 0.9981(17) \\
			&	2us 	 &   & 0.9969(8)  & 0.9979(17) \\
			&	4us 	 &   & 0.9965(9)  & 0.9975(17) \\\hline
\end{tabular}
\caption[Efficiency Factors DT]{\label{tab:LiveTimeFactorsDT} MTAS efficiency live time correction factors changing with respect to coincidence window. \todo[inline,color=ntb]{values to be checked again esp. for Zn.}}
\end{table}

\FloatBarrier

\subsection{Lilianna Notes}

Total live time for an isotope, $LTF$, is obtained from component-specific live times, $\ell_j$ ($j=C,I,O,M,P$) and associated component efficiencies $\epsilon_j$. These efficiencies denote the portion of events that are seen \emph{only} by that component. The total live time weighs $\ell_j$ by $\epsilon_j$, such that the first order live time correction is

\begin{equation}
    LTF^1 = \sum_j \ell_j \frac{\epsilon_j}{\epsilon_{tot}},
\end{equation}

where $\epsilon_{tot} = \sum_j\epsilon_j$. An nth order correction has the form

\begin{equation}
    LTF^n = \sum_{m=1}^{n-1} LTF^m + \sum_{\vec{j_n}\in J_n} \ell_{\vec{j_n}} \frac{\epsilon_{\vec{j_n}}}{\epsilon_{tot}},
\end{equation}

where $J_n = \{ \{j_i,..., j_n\} | j_1,...,j_n \in \{C, I, O, M, P\}, j_1\neq j_2\neq ...j_n \}$ and $\epsilon_{tot}\rightarrow \sum_n \sum_{\vec{j_n}} \epsilon_{\vec{j_n}}$. A set $J_n$ thus contains all non-repetitive, $n$-length combinations of MTAS components (e.g. $J_2$ has ${{5}\choose{2}} = 10$ elements). 

The $\epsilon_{tot}$ associated with the highest order correction represents the total system efficiency, as it takes into account all possible combinations of detections. For MTAS, the highest correction order is 5, so we define $LTF\equiv LTF^5$. The live time correction is then applied as a transformation to the efficiency such that

\begin{equation}
\varepsilon_i \longrightarrow \varepsilon_i \frac{LTF_{Mn}}{LTF_i},
\end{equation}

where $\varepsilon_i$ are Geant-scaled efficiencies (Table~\ref{tab:extrap_efficiency}) for $i=K, Zn$.

The total correction is dominated by first order terms, as dead time losses in one detector component do not result in a loss of overall efficiency if a different component of MTAS saw the same event.

All $\epsilon_{\vec{j_n}}$ are obtained from simulations, as scattering interactions in MTAS are $\mathcal{O}(100~ns)$, so coincidence-window ($\mathcal{O}(\mu s)$) effects do not need to be considered. $\ell_j$ ($j\equiv \vec{j_1}$) are obtained from Table~\ref{tab:CorrFactors} $\forall j\neq P$. The effect of the plug on total live time is negligible, primarily due to its count rates being an order of magnitude smaller than those in the rings of MTAS for the \Zn, \Mn, and \K\ experiments (see Table~\ref{tab:Rate_Table}). Additionally, weights $\epsilon_P$ for the plug are small. Negligibility of plug effects on live time is implemented by taking $\ell_P = 1 \pm 0$ (errorless, 100\% live time).

To obtain higher order corrections, $\ell_{\vec{j_n}}$ are inferred from aforementioned $\ell_j$. At the second order,

\begin{equation}
    \ell_{j_i,j_2} = 1 - (1-\ell_{j_1})(1-\ell_{j_2}),
\end{equation}

which is generalized to

\begin{equation}
    \ell_{\vec{j_n}} = 1 - \prod_n (1 - \ell_{j_n}).
\end{equation}

In obtaining $\epsilon_{\vec{j_n}}$ from simulations, energy thresholds are chosen for each MTAS component. Values $\epsilon_{\vec{j_n}}$ for the case of all thresholds being \keV{0} (not inclusive) are shown in Table~\ref{table:DT_correction_weights} for first order terms. Associated total live times are shown in Table~\ref{tab:DT:live_times}.

\begin{table}[ht]
\centering
%\resizebox{0.75\textwidth}{!}{
\begin{tabular}{cccc}
\hline
 Module   &    \multicolumn{3}{c}{ Weights for Correction}\\
 &  K  &	 Mn 	& Zn\\
 \hline
C   &	0.4429(2)	&	0.5817(2)	& 	0.5061(2)	\\
I   &   0.1893(1)	&	0.1358(1)	& 	0.1670(1)	\\
O   &    0.00297(2)	&	0.000658(8)	& 	0.00159(1)	\\
M   &	0.01126(3)	&	0.00432(2)	& 	0.00754(3)	\\
P   &   0.02169(5)  &   0.03490(6)   &   0.02719(5) \\
\hline
\end{tabular}%
%}
\caption{Efficiencies of separate MTAS components used to weigh live times, obtained for the 0-keV threshold case.}
\label{table:DT_correction_weights}
\end{table}

Although total corrections are highly-dominated by first-order terms, these weights only account for $\sim (65-70)\%$ of the total efficiency. The next largest weight is $\epsilon_{CI}\sim (15-20)\%$. Table~\ref{tab:LT_corrs_various_orders} displays the variation of $LTF_{Mn}/LTF_{i}$ with correction order, where correction order 5 accounts for the case that every component of MTAS detected an event. Past second order, it becomes difficult to discern variation at the precision of the associated error. As the \keV{1460} gamma of \K\ is more likely to make it past the center ring and induce detections in multiple components of MTAS than the \Zn\ (\keV{1115}) gamma, $LTF_{Mn}/LTF_{K}$ is more sensitive to higher-order corrections than $LTF_{Mn}/LTF_{Zn}$. A slight decrease in error is seen with higher-order corrections as more statistics are included in the calculation.

\begin{table}[ht]
    \centering
    \begin{tabular}{ccc}
    \hline
     Correction Order   &   \multicolumn{2}{c}{$LTF_{Mn}/LTF_{i}$ (1 $\mu$s CW)}    \\
        &   $i=K$ &   $i=Zn$  \\
    \hline
    1   &   1.00041(39) &   0.99955(33) \\
    2   &   1.00009(36) &   0.99957(32) \\
    3   &   1.00007(36) &   0.99957(32) \\ 
    4   &   1.00007(36) &   0.99957(32) \\
    5   &   1.00007(36) &   0.99957(32) \\
    \hline
    \end{tabular}
    \caption{Live time correction factors obtained using 0-keV thresholds at various orders of correction.}
    \label{tab:LT_corrs_various_orders}
\end{table}

\FloatBarrier
Combinations of component thresholds can in general lead to high variation in $\ell_{\vec{j_n}}$, up to an order of magnitude above its associated error. However, variation in sets of component thresholds has negligible effect on total correction factors $LTF_{Mn}/LTF_i$ as displayed for the 1-$\mu$s, $i=K$ case in Fig.~\ref{fig:DT_correction_v_threshold_K_1_us}. A similar trend is seen at the (2, 4)-$\mu$s CWs. For the case of $LTF_{Mn}/LTF_{Zn}$, variation is similarly minute, however this quantity increases with thresh\_C while decreasing with thresh\_P.

\begin{figure}[ht]
    \centering
    \includegraphics[width=0.9\textwidth]{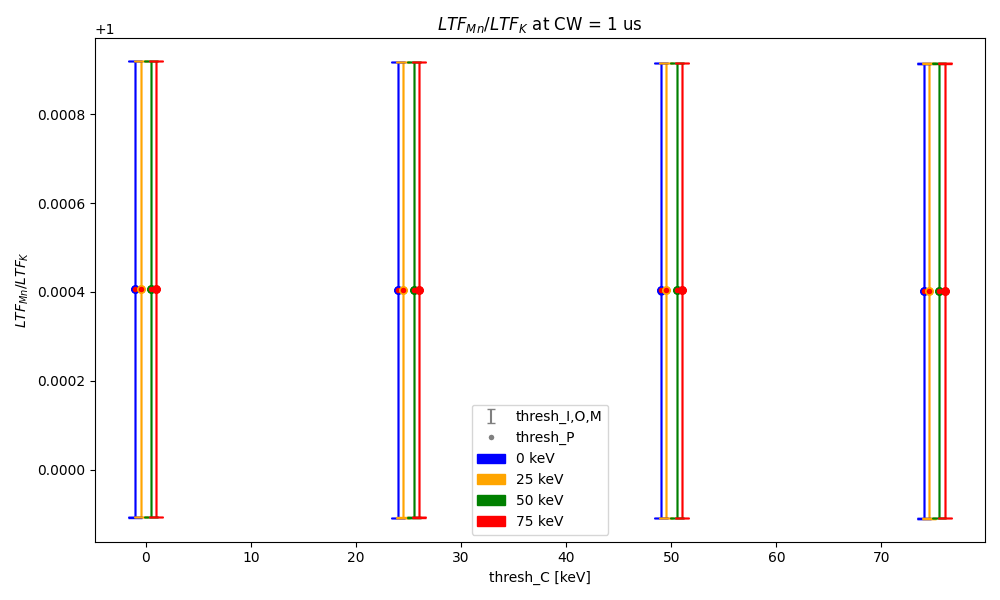}
    \includegraphics[width=0.9\textwidth]{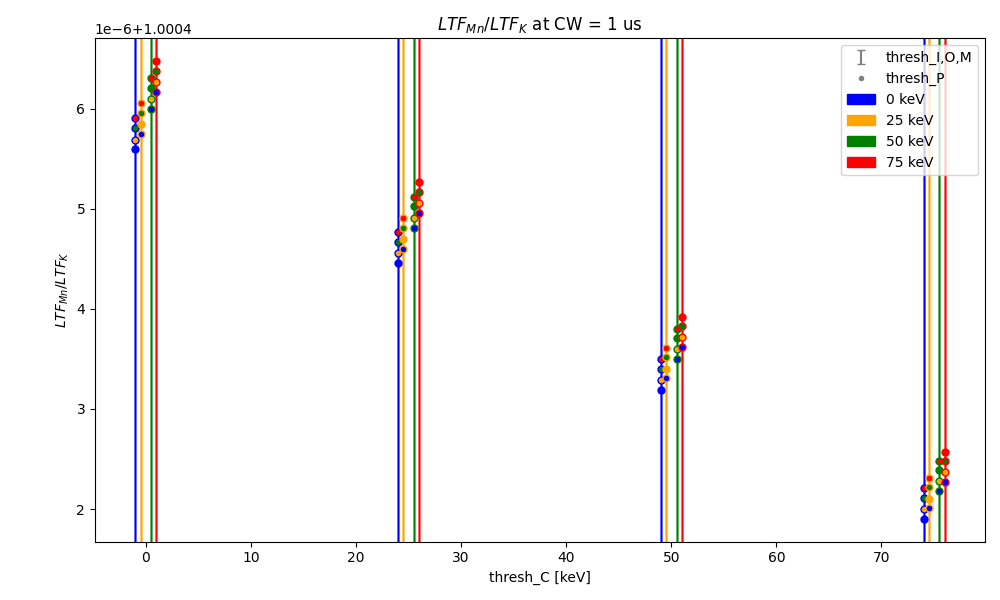}
    \caption{Variation in $LTF_{Mn}/LTF_K$ with MTAS component thresholds. Values are plotted against the threshold of the center ring, ``thresh\_C". For each data point, the errobar colour details the threshold applied to the inner, outer, and middle rings (``thresh\_I,O,M"), while the marker colour specifies the plug threshold (``thresh\_P"). Values were obtained at various combinations of the thresholds \keV{0}, \keV{25}, \keV{50}, \keV{75}. Data are offset from their true thresh\_C values for clarity. Errors are solely statistical.}
    \label{fig:DT_correction_v_threshold_K_1_us}
\end{figure}

It is seen that higher-rate experiments are associated with lower dead time. It is postulated that electronic noise dominates dead time and thus for a lower-rate experiment a noisy waveform being more significant results in higher dead time relative to a higher-rate experiment. This postulation implies a lack of CW-dependency of live times, which is, minimally, not in contention with the within 2$\sigma$ agreement across CWs seen in Table~\ref{tab:DT:live_times}. However. domination of noise effects on live time implies a correlation between $LTF_i$ values. In this regime, errors associated with $LTF_{Mn}/LTF_{i}$ may be considered upper limits on the errors, as no covariance terms are involved in their calculation.

\subsubsection{Effect of $\ell_P$}

Table~\ref{tab:effect_ell_P_on_DT} shows correction factors obtained for the usual $\ell_P = 1.00(0)$ case and those obtained taking $\ell_P = 0.990(5)$. The variation in correction factor is a fraction of the associated error. A 0.005 error on $\ell_P$ increases the (usual) total error by $\sim (20-30)\%$.

\begin{table}[ht]
    \centering
    \begin{tabular}{ccccc}
    \hline
     CW &   \multicolumn{2}{c}{$LTF_{Mn}/LTF_K$}  &   \multicolumn{2}{c}{$LTF_{Mn}/LTF_{Zn}$}  \\
        &   $\ell_P = 1.00(0)$  &   $\ell_P = 0.990(5)$   &   $\ell_P = 1.00(0)$  &   $\ell_P = 0.990(5)$ \\
     \hline
     1  &   1.000072(356)    &   1.000072(425)  &   0.999569(318)   &   0.999569(404)   \\
     2  &   1.000102(356)   &   1.00010(425)   &   0.999577(318)   &   0.999577(404)   \\
     4  &   1.000075(356)   &   1.000075(425)   &   0.999615(326)   &   0.999615(410)   \\
     \hline
    \end{tabular}
    \caption{Variation in $LTF_{Mn}/LTF_i$ with decrease in $\ell_P$ and introduction of an associated error.}
    \label{tab:effect_ell_P_on_DT}
\end{table}

Since there are 12 PMTs connected to a single crystal, it is expected that all 12 should trigger simultaneously. If there is a center multiplicity less than 12, the event energy is scaled by 12 divided by the multiplicity. The energy of the central modules are adjusted further in the gain match procedure. Therefore the dead time resulting from losing channels in the central module is not effecting the efficiency.

\clearpage
