# Supplementary material for: A novel experimental system for the KDK measurement of the $^{40}$K decay scheme relevant for rare event searches
Source: arXiv:2012.15232 source file (2021-07-27)
Supplement: Supplementary file 4 [file Appendix_KCl_Calculation.tex]

\section{KCl Thickness Calculation (Not For Publications) \label{App:KCl Calculations}}

This appendix is to supplement the information in Section~\ref{subsubsec:K40Source}.
The thickness of the KCl films produced was characterized by scanning electron microscopy (SEM) analysis. Two KCl films were analyzed, one with 1.5(1) mg of natural KCl and the other with 1.45(12) mg of 3.15$\%$ enriched KCl. The thickness of the natural KCl film was measured to be 11(1) $\mu$m. This is an average thickness of 20 measurements. It is noted that the calculated thickness of 1.5 mg KCl uniformly distributed in a circle of about 1-cm diameter is 9.7(6) $\mu$m, which is statistically consistent with the SEM measurement.

The volume (cm$^3$) of a cylinder is given by

\begin{equation}\label{Eqn:Vol_Cylinder}
    V = \pi r^2 h,
\end{equation}
where r is the radius (cm) and h is the height (cm). Assuming that the KCl particles are uniformly distributed in the cylinder eqn.~\ref{Eqn:Vol_Cylinder} can be modified as
\begin{equation}\label{Eqn:Vol_Cylinder_mod}
    \frac{m}{d} = \pi r^2 h,
\end{equation}
where $m$ is the mass of KCl deposited and $d$ is the density of KCl (1.98 g/cm$^3$). Rearranging Eqn.~\ref{Eqn:Vol_Cylinder_mod} for the height gives
\begin{equation}\label{Eqn:Vol_Cylinder_h}
    h = \frac{m}{d \pi r^2}.
\end{equation}
With a mass of 1.5(1)mg Eqn.~\ref{Eqn:Vol_Cylinder_h} gives h = 9.7(6) $\mu$m. The ratio of SEM measured film thickness to calculated film thickness is 11(1)/9.7(6) = 1.14(13). 

The final KCl source (created from 16.1(6)$\%$ enriched \K ) had a total deposition of 0.69(11)mg of KCl. The thickness of the source was not measured using the SEM. It was instead estimated using Eqn~\ref{Eqn:Vol_Cylinder_h} (4.44(71)$\mu$m) and the SEM-to-calculated film thickness ratio (\textbf{4.44(71)$\times$1.14(13)=5.1(9)}).

\clearpage
