# Supplementary material for: A novel experimental system for the KDK measurement of the $^{40}$K decay scheme relevant for rare event searches
Source: arXiv:2012.15232 source file (2021-07-27)
Supplement: Supplementary file 5 [file Appendix_KSI.tex]

\section{KSI appendix (Not For Publication)}

Activation of the Eu dopend within KSI presents a few challenges when calibrating in the low energy region below 80 keV. The presence of auger electrons as well as conversion electrons in the same peak locations as the X-rays creates large uncertainties around the true mean of the peak. The 40 and 46 keV peaks in the Eu activation coincidence spectra look to be in the right location based on other calibration points, however their relative intensities do not seem to be correct. The intensity of the 46 keV point should be several times less than that of the 40 keV peak according the the NNDC data base but we see the opposite in the spectra. One potential reason for this discrepancy is the addition of the 32 keV auger electron depositing energy in the location of the 40 and 46 keV X-rays. Another theory is what is assumed to be the 40 keV peak is actually the 46 keV peak and the 32 keV auger electron is depositing its energy in the 40 keV range. This however does not agree with the \Cs\ spectra with a 32 keV X-ray lower in the curve. In order to clear up these discrepancies, an in depth study into auger electron interaction within the sensing volume would need to be conducted, which is beyond the scope of this collaboration. We will continue with the original assumption that the two Eu peaks in question are in fact the 40 and 46 keV X-ray peaks and omit the 46 keV peak due to the relative intensity not agreeing with expected intensity. The remaining 4 calibration points are sufficient in characterizing the light yield of KSI, especially in the 2-6 keV energy range in question, however, since the 5 - 6 keV peak from Eu is convolved with Auger electrons around the same energy, assigning an energy to the peak is not possible for reasons stated previously. In this case, the peak is used to confirm the location of the \K\ 3 keV peak and not as a calibration point.

\begin{figure}[ht]
  \centering
  \includegraphics[width=1.0\linewidth]{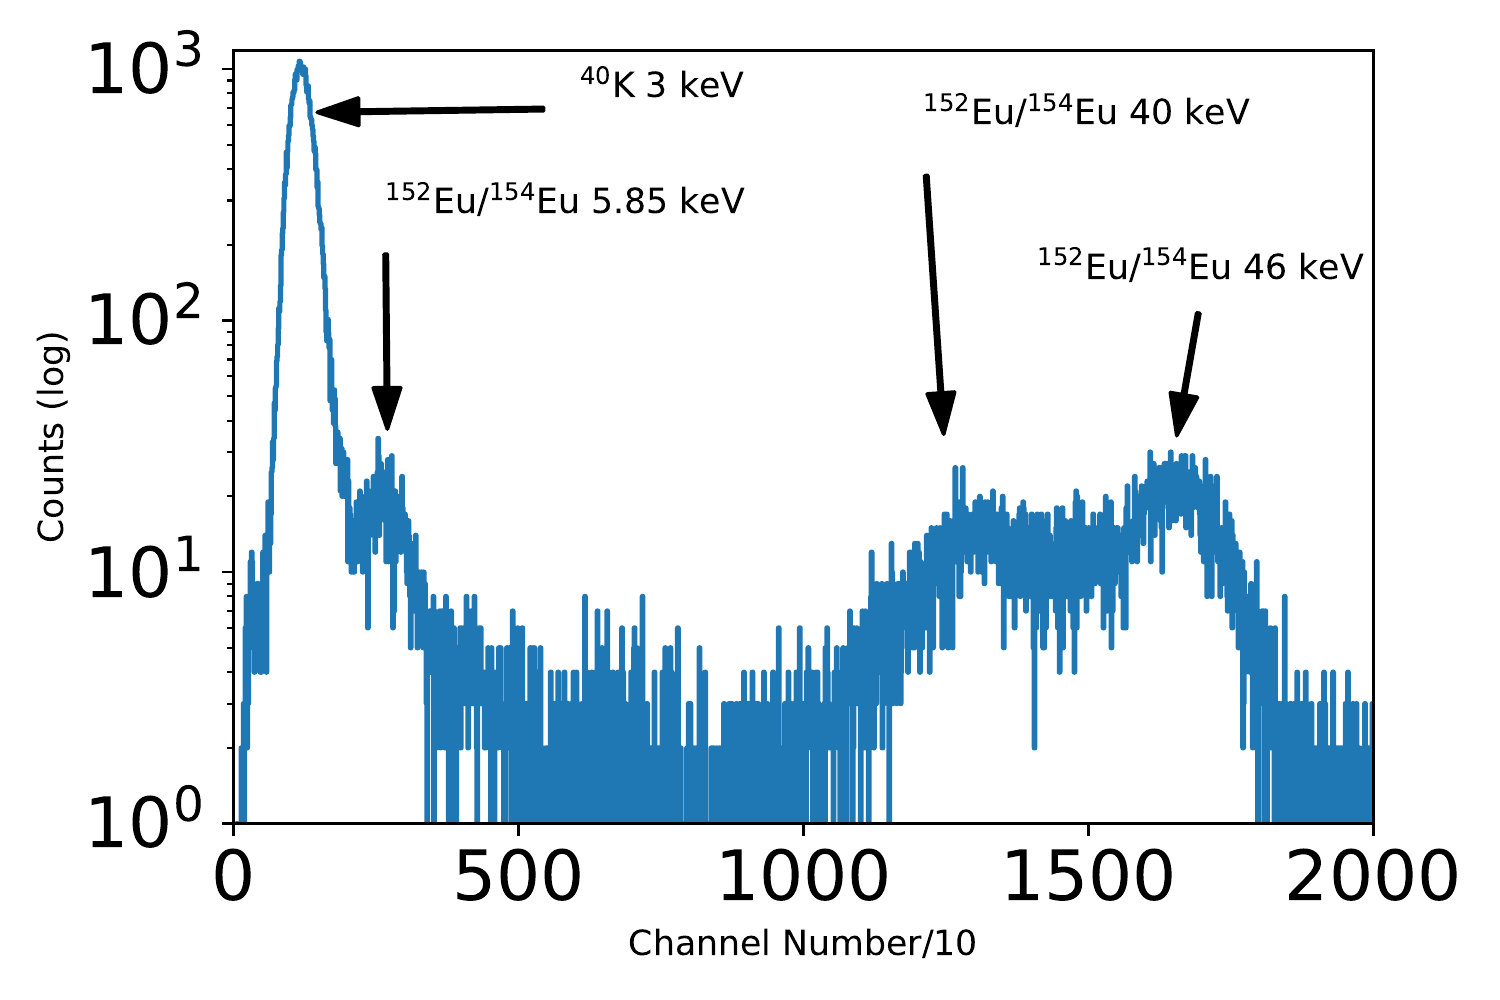}
	\caption{\label{Fig:Eu_activation_Plot_full.pdf}Full Eu activation coincidence spectra including the 46 keV point.}
\end{figure}

\begin{figure}[h]
  \centering
  \includegraphics[width=1.0\linewidth]{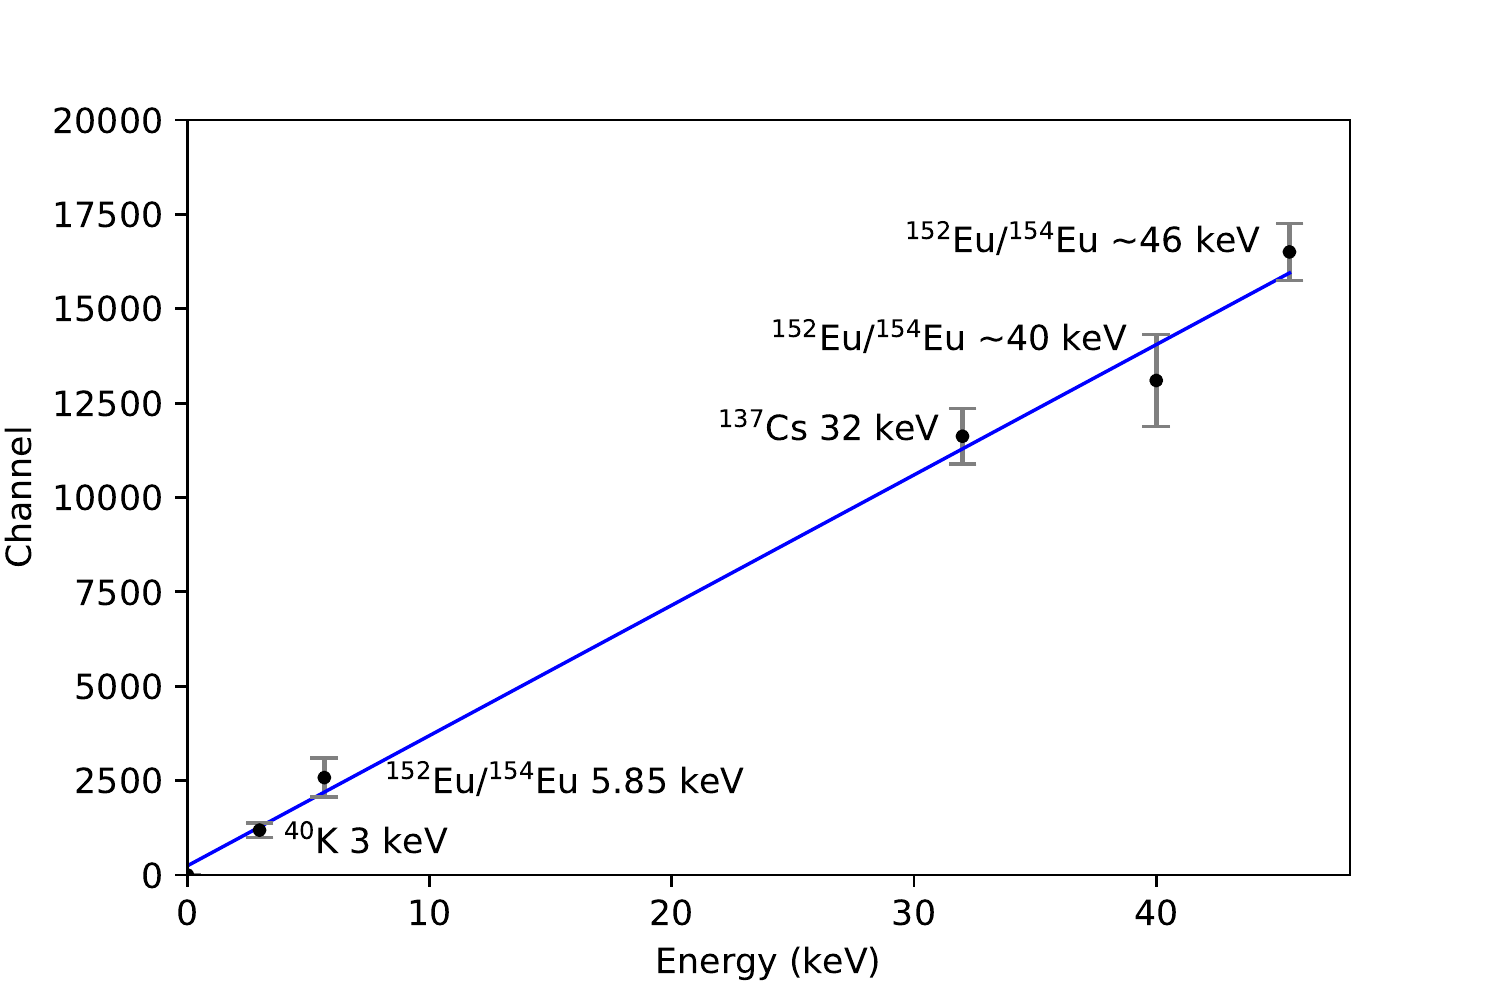}
	\caption{\label{Fig:KSI_Eu_calibration_full.pdf}The calibration curve for the low energy region of KSI shown with error bars calculated as the standard deviation of the mean for the corresponding sources, including the 46 keV extrapolated point.}
\end{figure}
